# Supplementary material for: CoV: Chain-of-View Prompting for Spatial Reasoning
Source: arXiv:2601.05172 source file (2026-01-09)
Supplement: Supplementary file 1 [file cov_supp-crop.pdf]

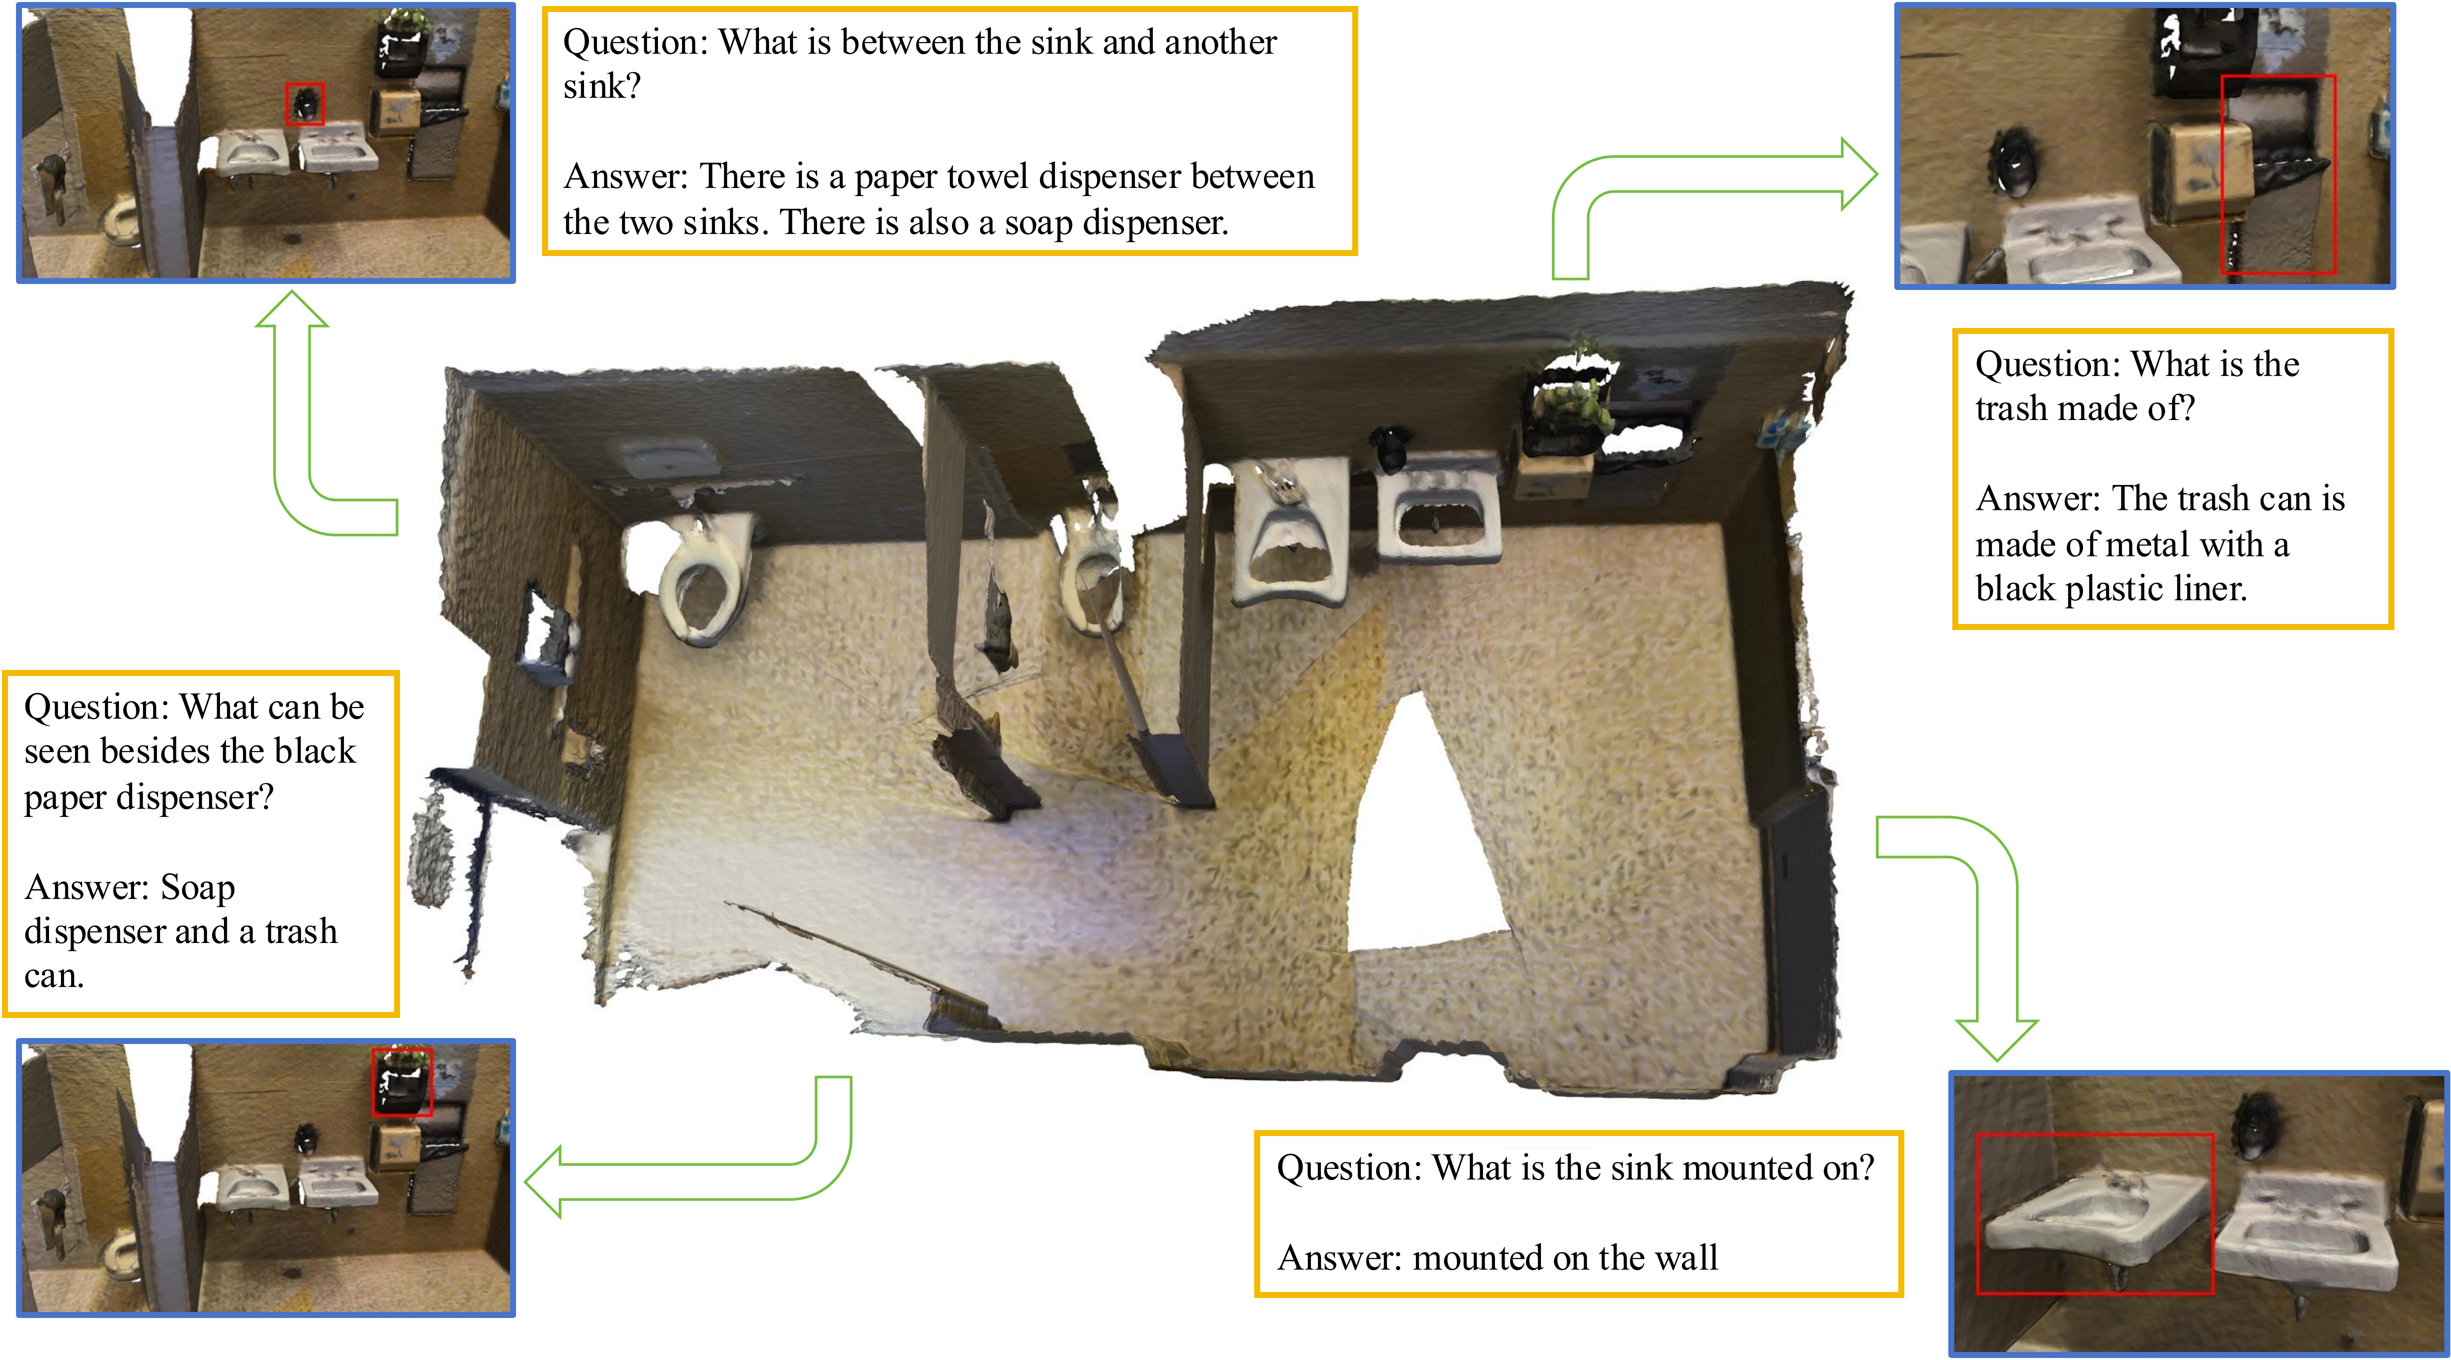
Question: What is between the sink and another sink?
Answer: There is a paper towel dispenser between the two sinks. There is also a soap dispenser.
Question: What is the trash made of?
Answer: The trash can is made of metal with a black plastic liner.
Question: What can be seen besides the black paper dispenser?
Answer: Soap dispenser and a trash can.
Question: What is the sink mounted on?
Answer: mounted on the wall

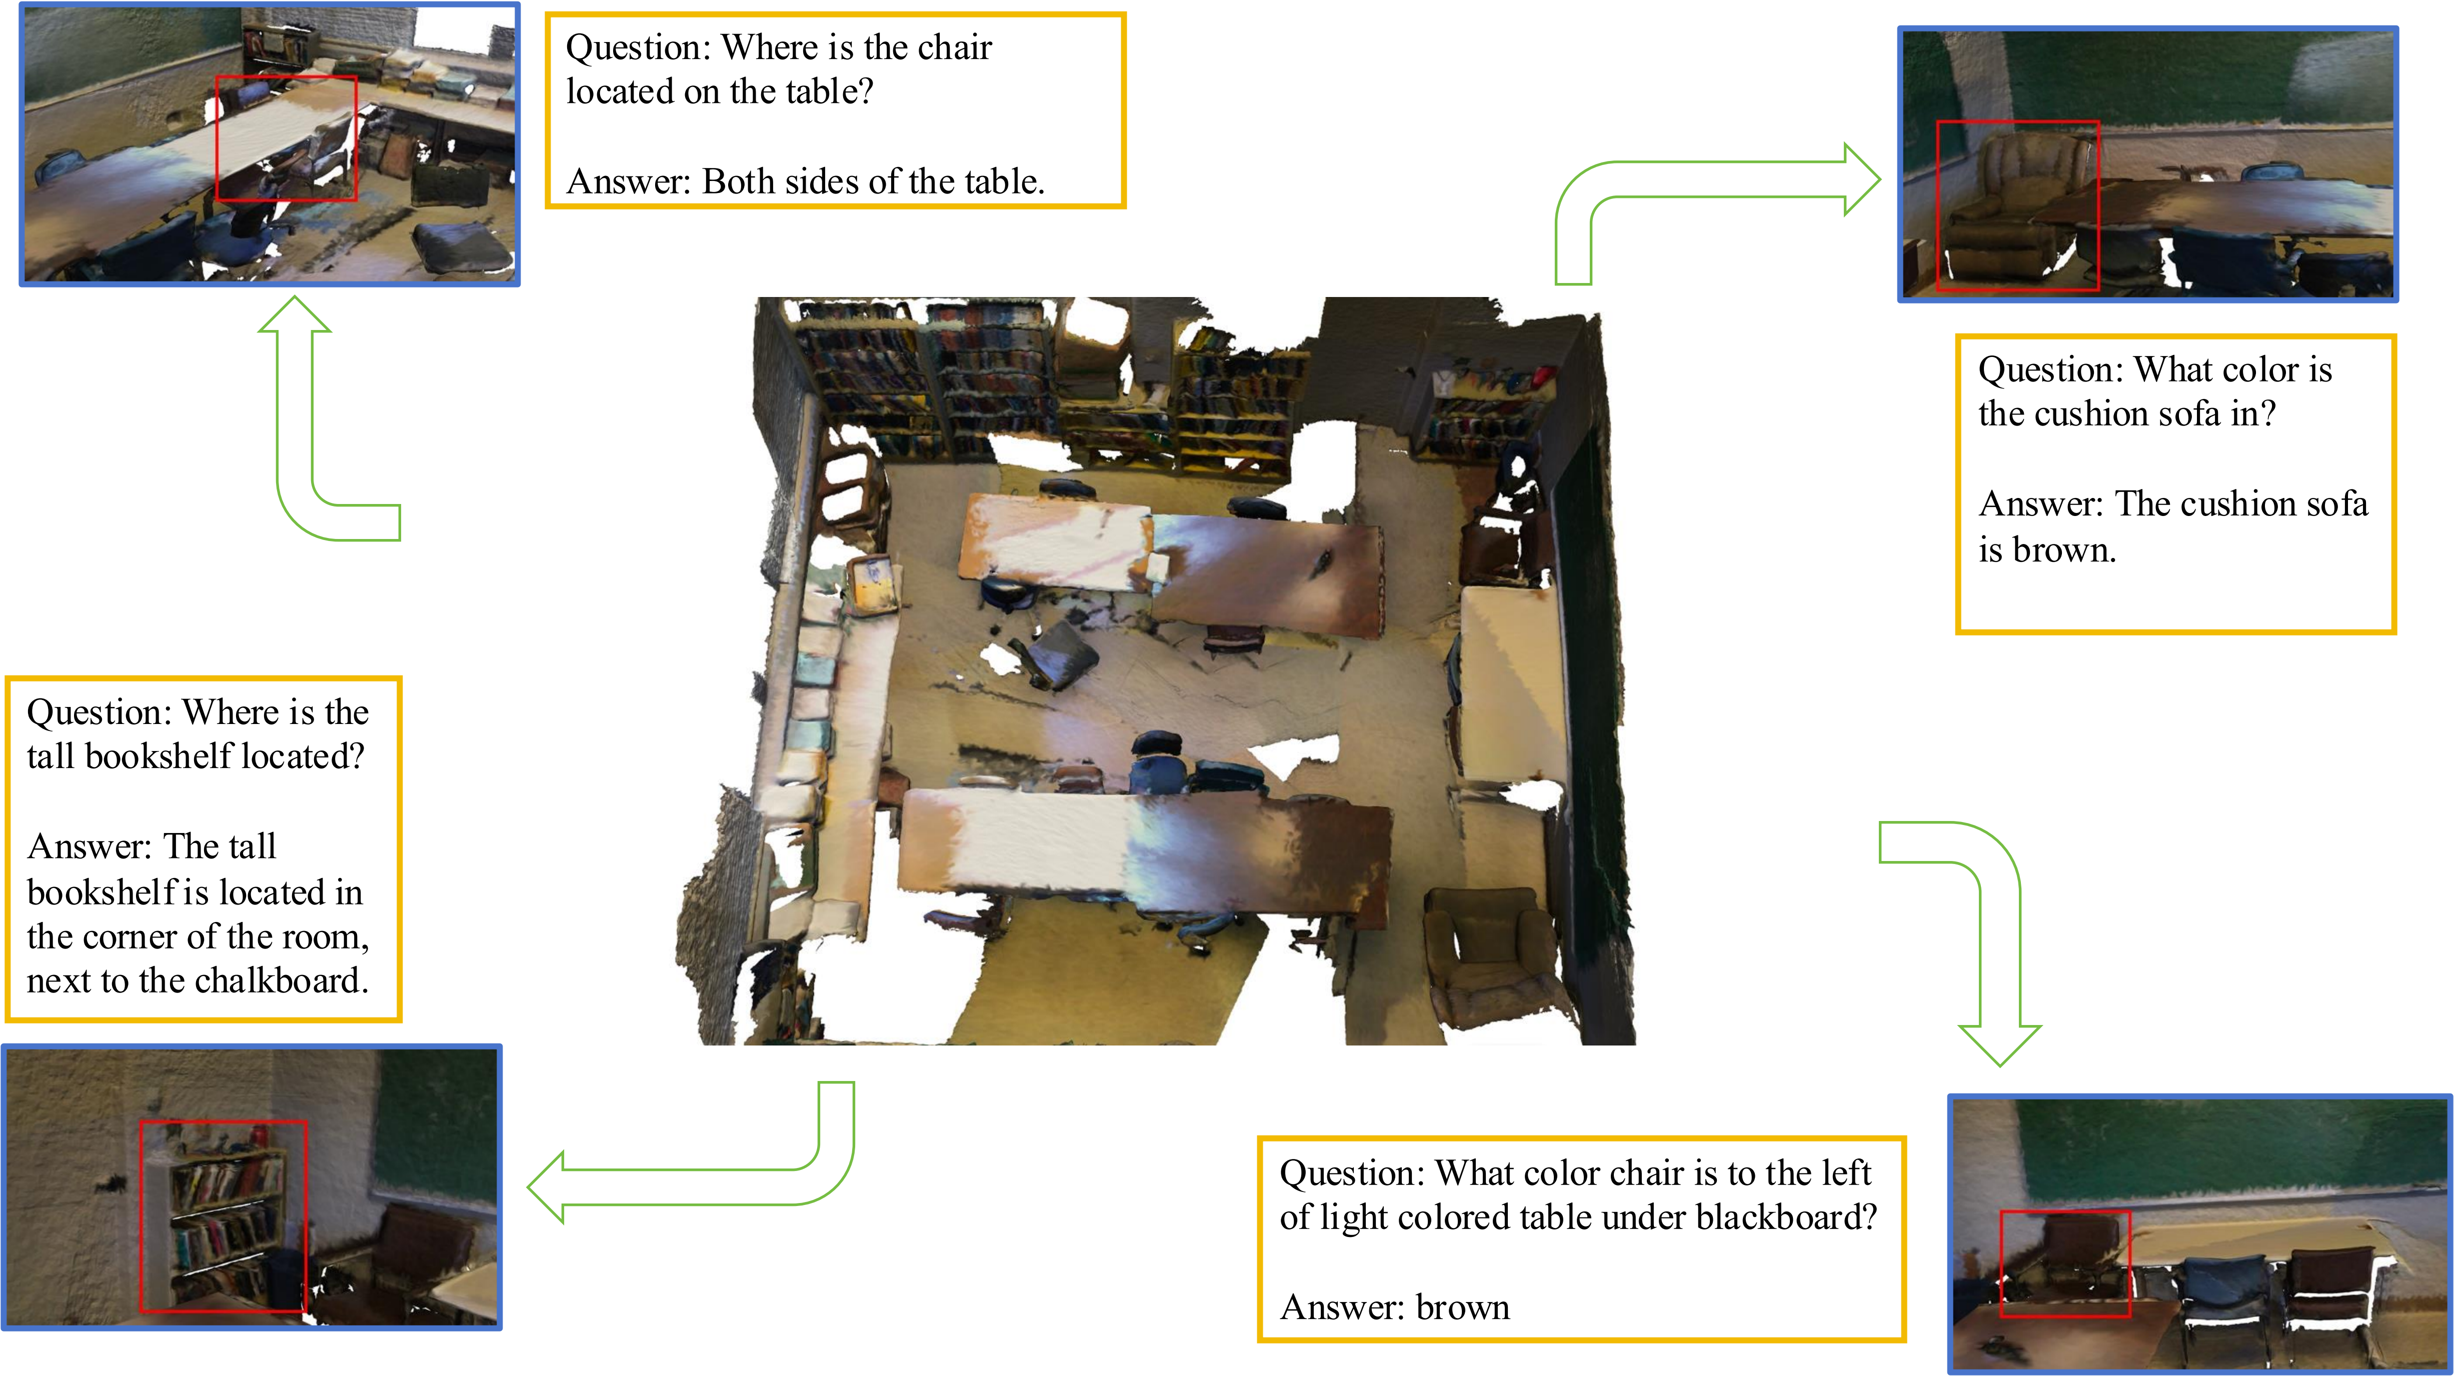
Question: Where is the chair located on the table?
Answer: Both sides of the table.
Question: What color is the cushion sofa in?
Answer: The cushion sofa is brown.
Question: Where is the tall bookshelf located?
Answer: The tall bookshelf is located in the corner of the room, next to the chalkboard.
Question: What color chair is to the left of light colored table under blackboard?
Answer: brown

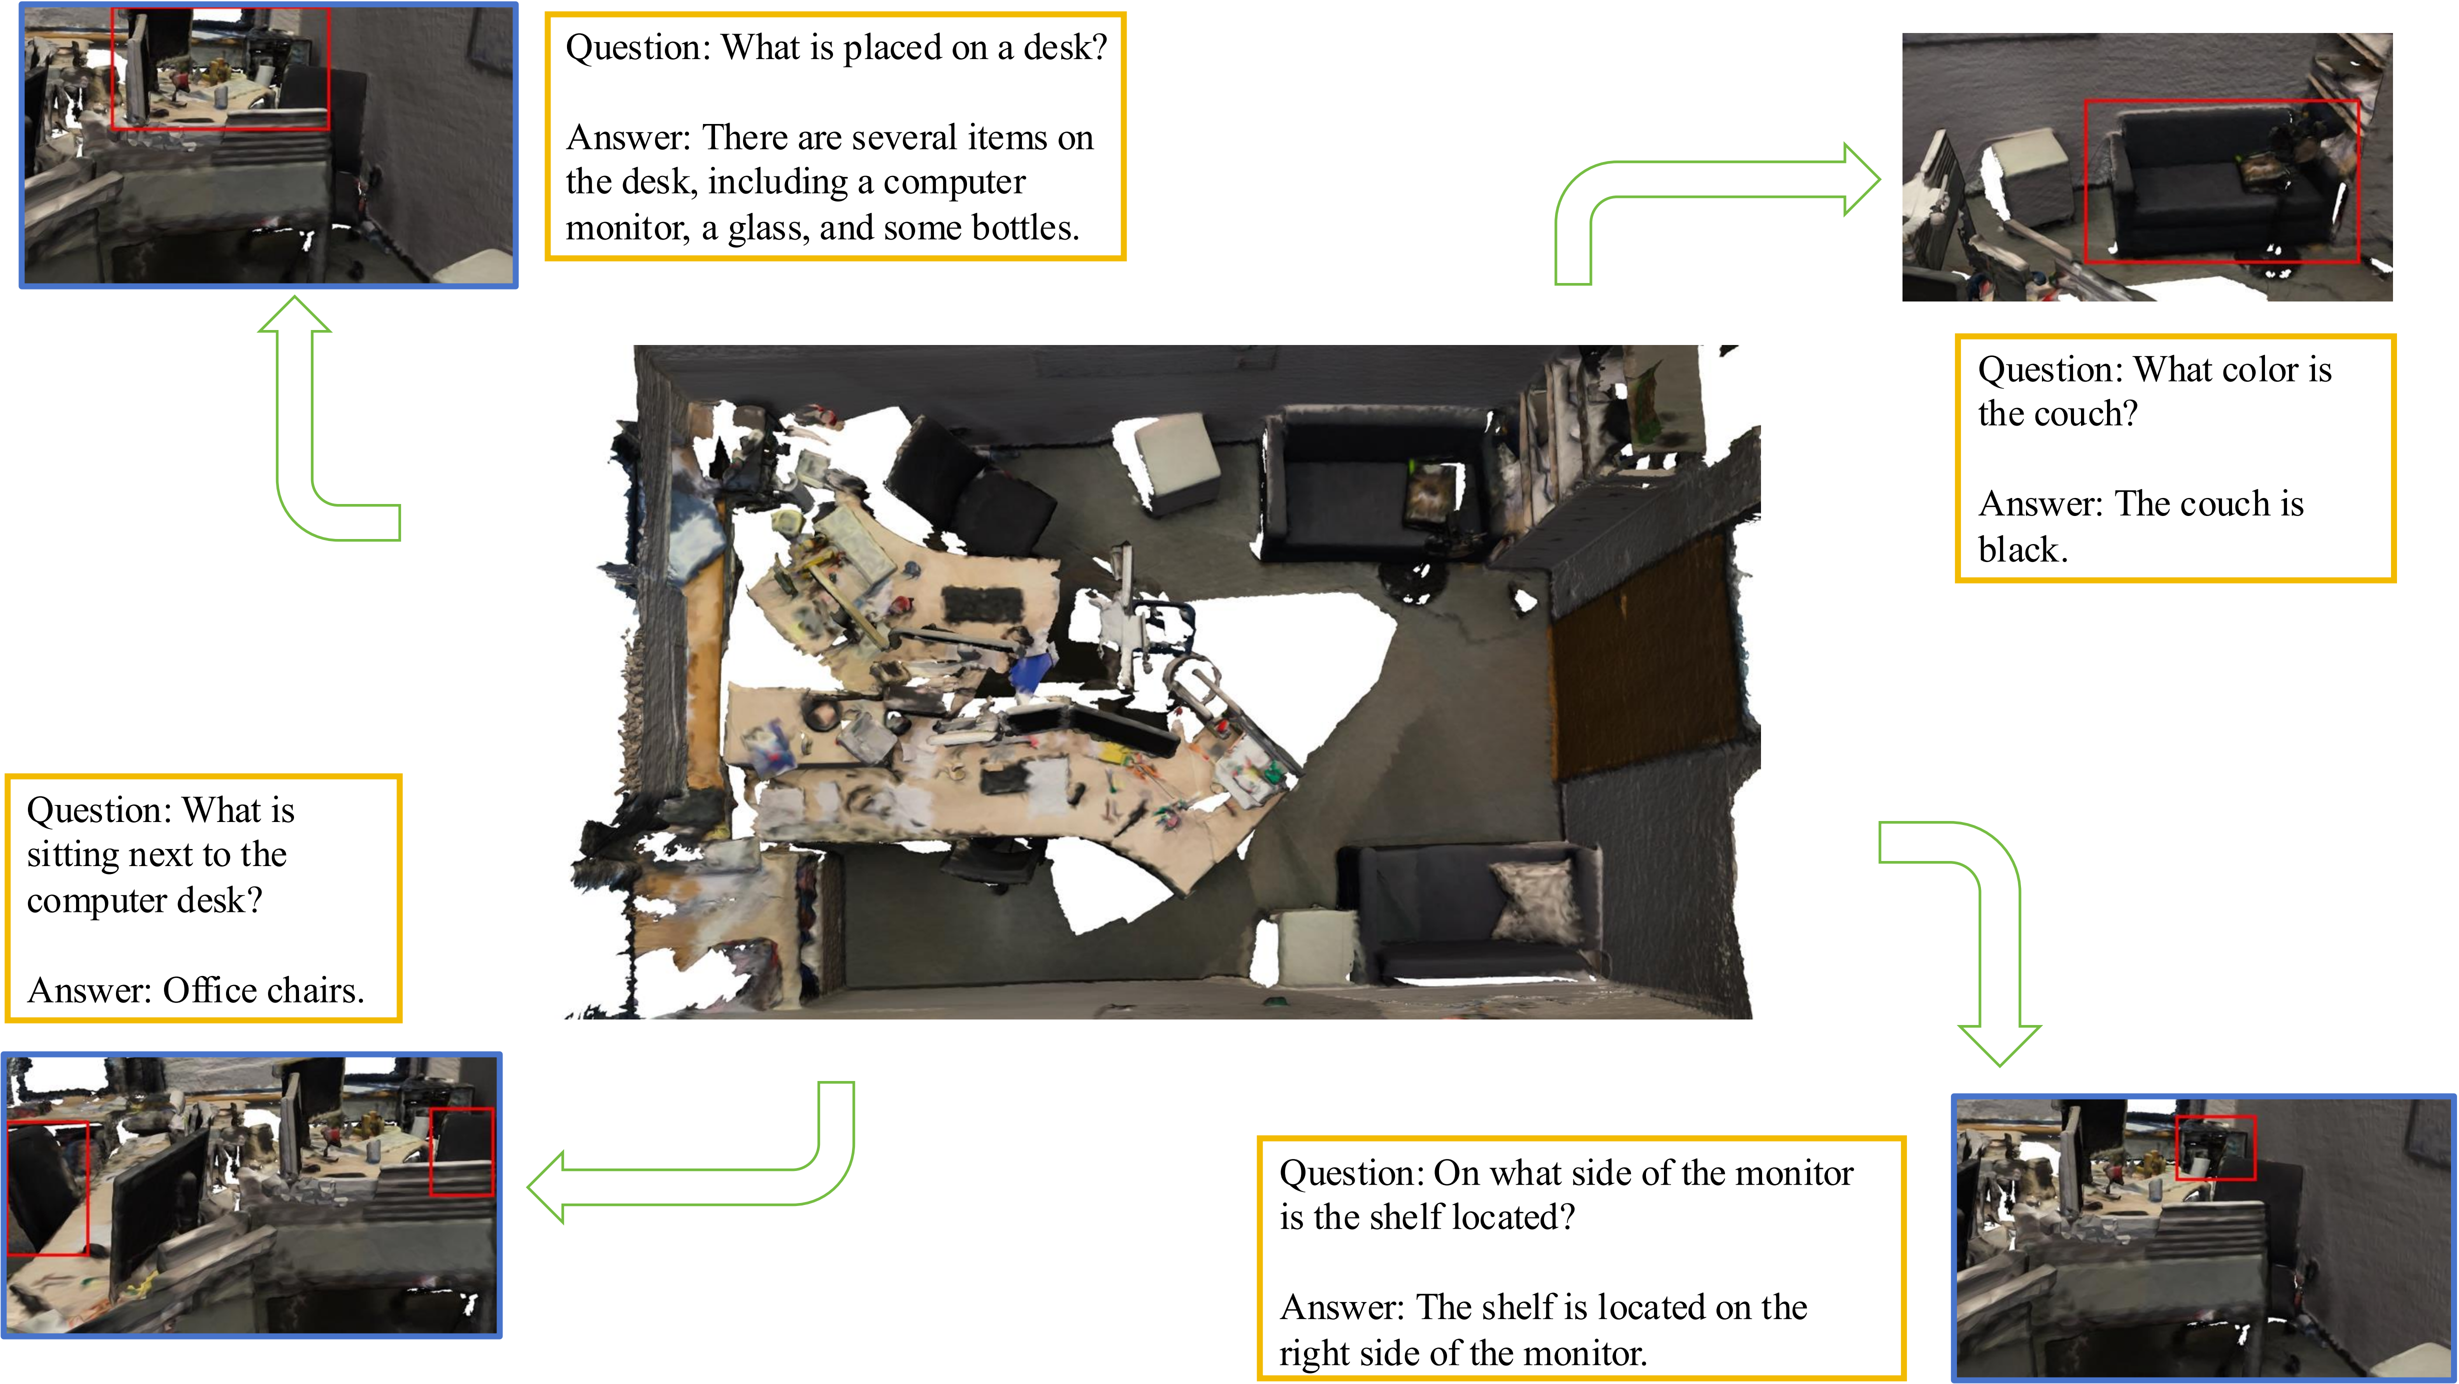

Question: What is placed on a desk?
Answer: There are several items on the desk, including a computer monitor, a glass, and some bottles.
Question: What color is the couch?
Answer: The couch is black.
Question: What is sitting next to the computer desk?
Answer: Office chairs.
Question: On what side of the monitor is the shelf located?
Answer: The shelf is located on the right side of the monitor.

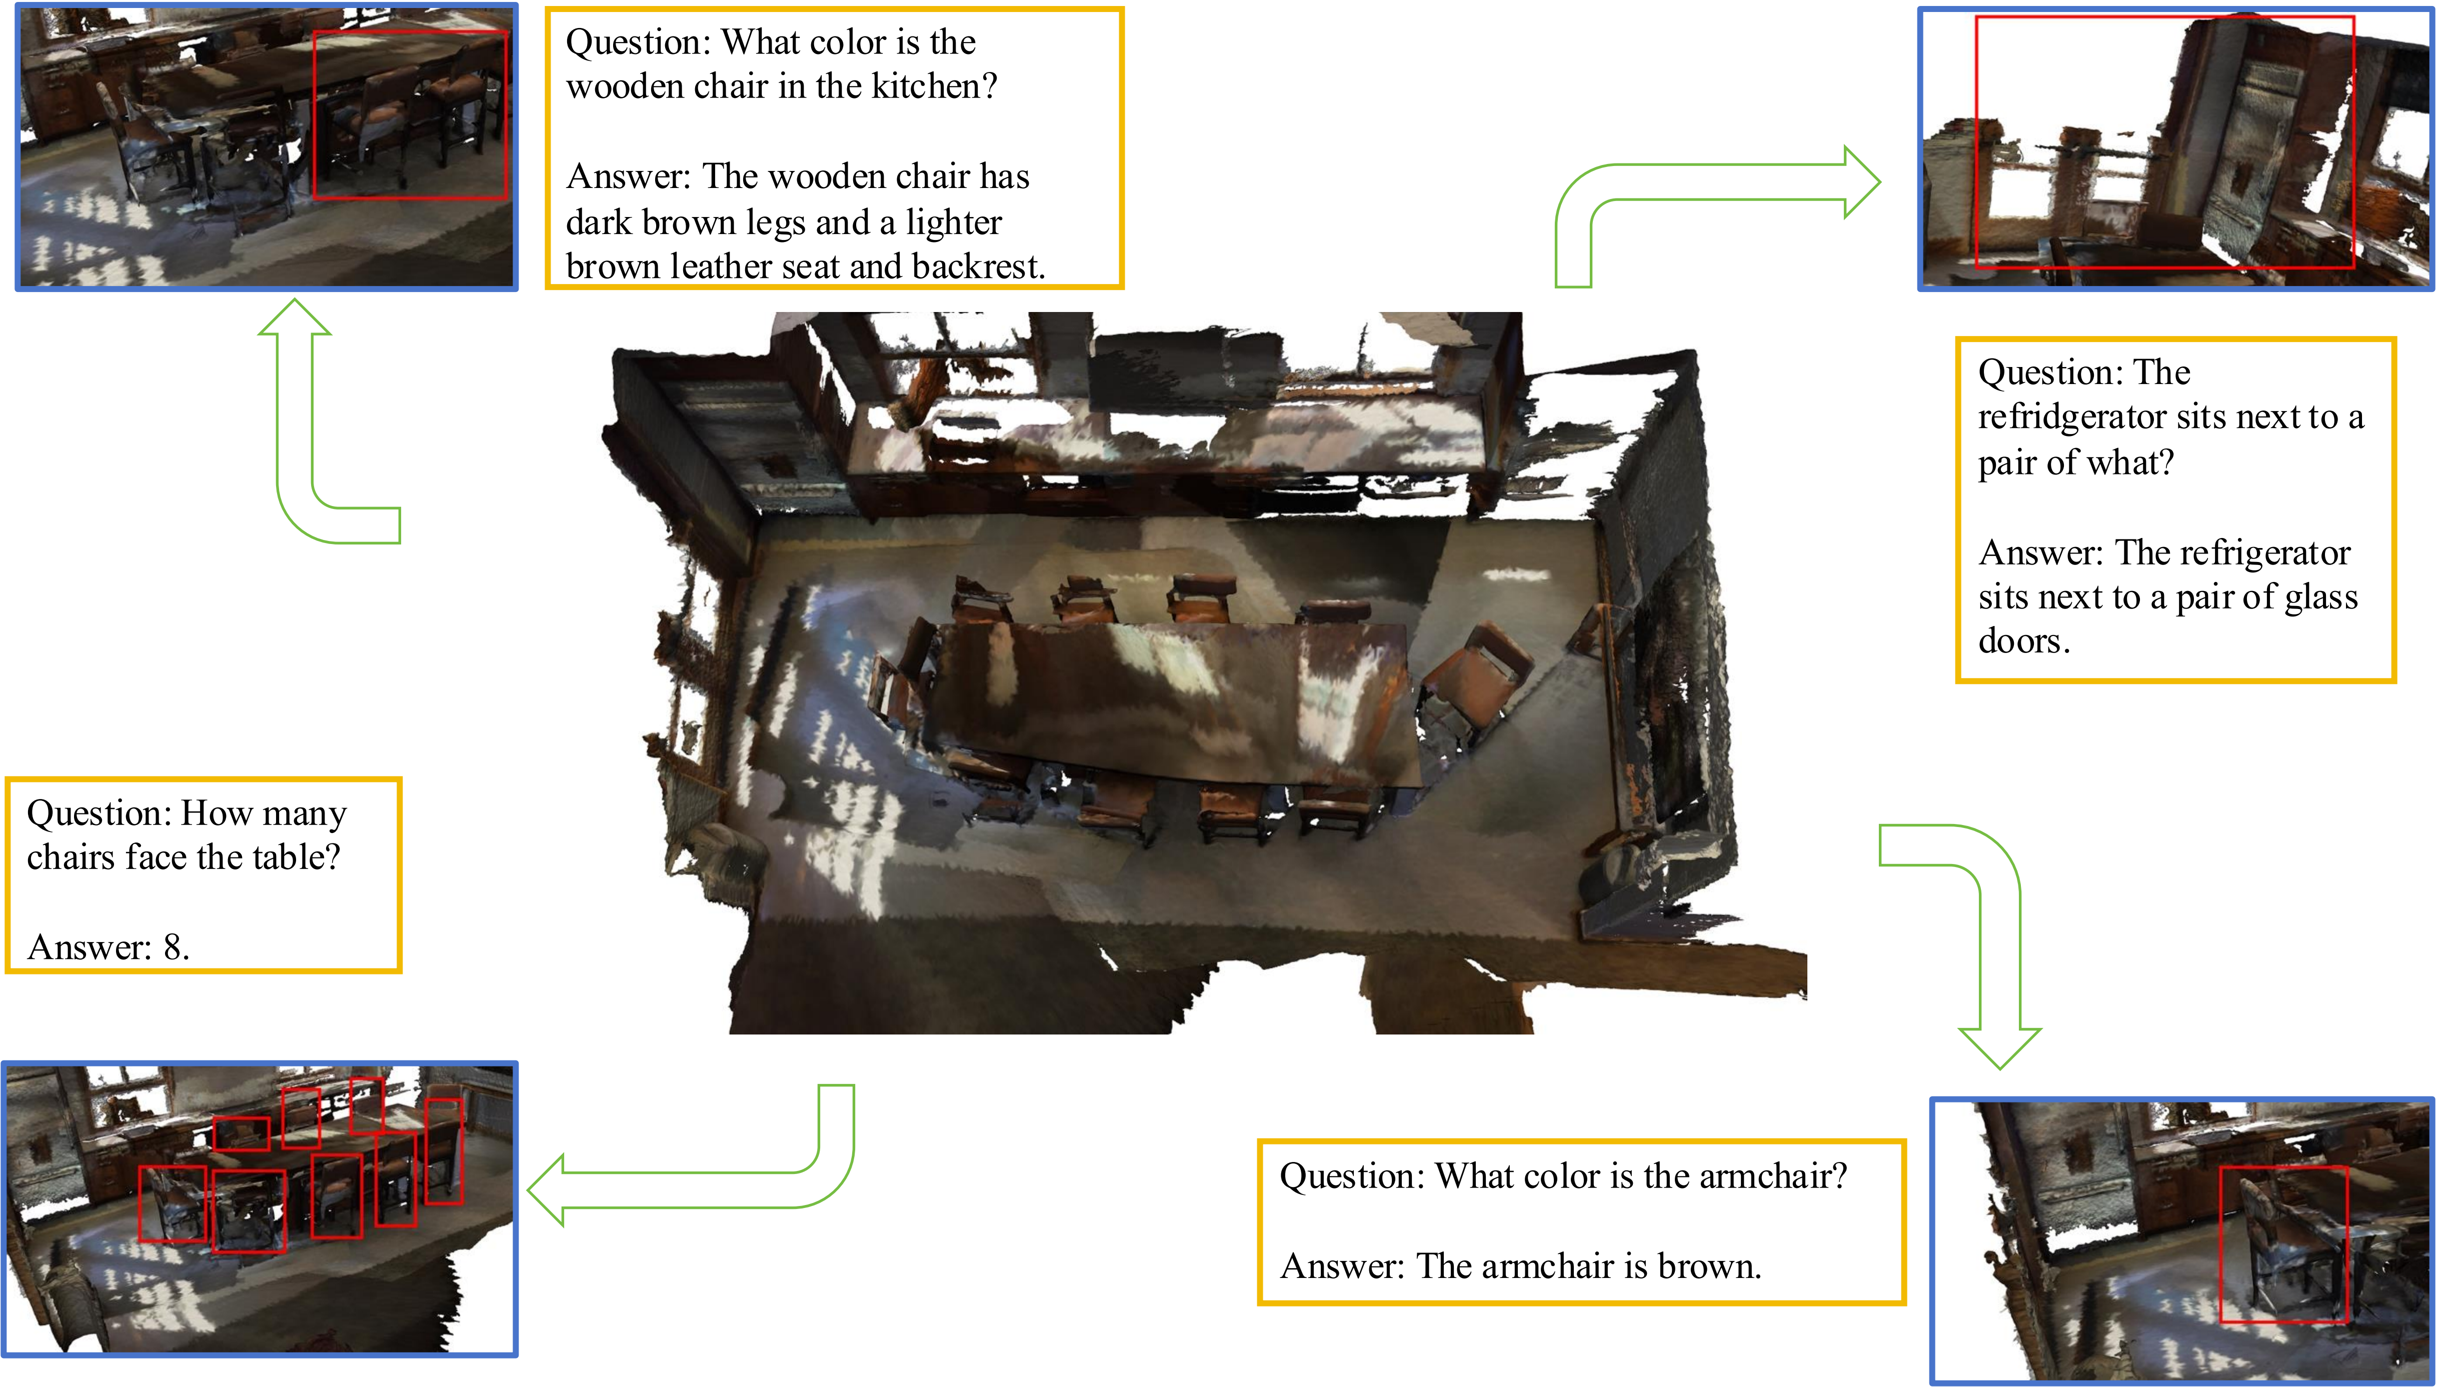
Question: What color is the wooden chair in the kitchen?
Answer: The wooden chair has dark brown legs and a lighter brown leather seat and backrest.
Question: The refridgerator sits next to a pair of what?
Answer: The refrigerator sits next to a pair of glass doors.
Question: How many chairs face the table?
Answer: 8.
Question: What color is the armchair?
Answer: The armchair is brown.
